# Supplementary material for: Effective Mutation Rate Adaptation through Group Elite Selection
Source: arXiv:2204.04817 source file (2022-04-11)
Supplement: Supplementary file 1 [file main_appendix.tex]

%%
%% This is file `sample-sigconf.tex',
%% generated with the docstrip utility.
%%
%% The original source files were:
%%
%% samples.dtx  (with options: `sigconf')
%% 
%% IMPORTANT NOTICE:
%% 
%% For the copyright see the source file.
%% 
%% Any modified versions of this file must be renamed
%% with new filenames distinct from sample-sigconf.tex.
%% 
%% For distribution of the original source see the terms
%% for copying and modification in the file samples.dtx.
%% 
%% This generated file may be distributed as long as the
%% original source files, as listed above, are part of the
%% same distribution. (The sources need not necessarily be
%% in the same archive or directory.)
%%
%%
%% Commands for TeXCount
%TC:macro \cite [option:text,text]
%TC:macro \citep [option:text,text]
%TC:macro \citet [option:text,text]
%TC:envir table 0 1
%TC:envir table* 0 1
%TC:envir tabular [ignore] word
%TC:envir displaymath 0 word
%TC:envir math 0 word
%TC:envir comment 0 0
%%
%%
%% The first command in your LaTeX source must be the \documentclass command.
\documentclass[sigconf]{acmart}

%%
%% \BibTeX command to typeset BibTeX logo in the docs
\AtBeginDocument{%
  \providecommand\BibTeX{{%
    \normalfont B\kern-0.5em{\scshape i\kern-0.25em b}\kern-0.8em\TeX}}}

%% Rights management information.  This information is sent to you
%% when you complete the rights form.  These commands have SAMPLE
%% values in them; it is your responsibility as an author to replace
%% the commands and values with those provided to you when you
%% complete the rights form.
\setcopyright{acmcopyright}
\copyrightyear{2022}
\acmYear{2022}
\acmDOI{10.1145/1122445.1122456}

%% These commands are for a PROCEEDINGS abstract or paper.
\acmConference[Woodstock '18]{Woodstock '18: ACM Symposium on Neural
  Gaze Detection}{June 03--05, 2018}{Woodstock, NY}
\acmBooktitle{Woodstock '18: ACM Symposium on Neural Gaze Detection,
  June 03--05, 2018, Woodstock, NY}
\acmPrice{15.00}
\acmISBN{978-1-4503-XXXX-X/18/06}

\usepackage{algorithm}
\usepackage{algorithmic}

\usepackage{mathtools}
% \usepackage{times}  % DO NOT CHANGE THIS
% \usepackage{mathtools}

% \DeclarePairedDelimiter\floor{\lfloor}{\rfloor}

% \usepackage{helvet}  % DO NOT CHANGE THIS
% \usepackage{courier}  % DO NOT CHANGE THIS
% \usepackage[hyphens]{url}  % DO NOT CHANGE THIS
% \usepackage{graphicx} % DO NOT CHANGE THIS
% \urlstyle{rm} % DO NOT CHANGE THIS
% \def\UrlFont{\rm}  % DO NOT CHANGE THIS
% \usepackage{natbib}  % DO NOT CHANGE THIS AND DO NOT ADD ANY OPTIONS TO IT
% \usepackage{caption} % DO NOT CHANGE THIS AND DO NOT ADD ANY OPTIONS TO IT
% \DeclareCaptionStyle{ruled}{labelfont=normalfont,labelsep=colon,strut=off} % DO NOT CHANGE THIS
% \frenchspacing  % DO NOT CHANGE THIS
% \setlength{\pdfpagewidth}{8.5in}  % DO NOT CHANGE THIS
% \setlength{\pdfpageheight}{11in}  % DO NOT CHANGE THIS
%
% These are recommended to typeset algorithms but not required. See the subsubsection on algorithms. Remove them if you don't have algorithms in your paper.

%\usepackage{asmmath}

% MINE (Akarsh)
\usepackage{amsfonts}
\usepackage{multirow}
\usepackage{siunitx}
\usepackage{amsmath}
\usepackage{amssymb}
\usepackage{amsthm}
\usepackage{siunitx}
\usepackage{booktabs}

\usepackage{algorithmic}

% expected value
% expected value
% expected value
\usepackage{mathtools}

%%
%% Submission ID.
%% Use this when submitting an article to a sponsored event. You'll
%% receive a unique submission ID from the organizers
%% of the event, and this ID should be used as the parameter to this command.
%%\acmSubmissionID{123-A56-BU3}

%%
%% The majority of ACM publications use numbered citations and
%% references.  The command \citestyle{authoryear} switches to the
%% "author year" style.
%%
%% If you are preparing content for an event
%% sponsored by ACM SIGGRAPH, you must use the "author year" style of
%% citations and references.
%% Uncommenting
%% the next command will enable that style.
%%\citestyle{acmauthoryear}

%%
%% end of the preamble, start of the body of the document source.
\begin{document}

%%
%% The "title" command has an optional parameter,
%% allowing the author to define a "short title" to be used in page headers.
\title{
%Adapting to the Optimal Mutation Rate in Genetic Algorithms with Group Elite Selection
Appendix of Effective Mutation Rate Adaptation\\through Group Elite Selection
% Addressing premature convergence in
% self-adaptive genetic algorithms 
% with Group Elite Selection
% How evolution may be adapting mutation 
% rates for the long-term 
% Effective/Long-term Mutation Rate Adaptation through Group Elite Selection
% Optimal Mutation Rate for Evolutionary Computation
}

%%
%% The "author" command and its associated commands are used to define
%% the authors and their affiliations.
%% Of note is the shared affiliation of the first two authors, and the
%% "authornote" and "authornotemark" commands
%% used to denote shared contribution to the research.

% \author{Akarsh Kumar}
% \affiliation{%
%   \institution{The University of Texas at Austin}
%   \streetaddress{1 Th{\o}rv{\"a}ld Circle}
%   \city{Austin} \state{Texas} \country{USA}
%   }
% \email{akarshkumar0101@gmail.com}

% \author{Bo Liu}
% \affiliation{%
%   \institution{The University of Texas at Austin}
%   \city{Austin} \state{Texas} \country{USA}
% }
% \email{bliu@cs.utexas.edu}

% \author{Risto Miikkulainen}
% \affiliation{%
%   \institution{The University of Texas at Austin}
%   \institution{and Cognizant AI Labs}
%   \streetaddress{30 Shuangqing Rd}
%   \city{Austin} \state{Texas} \country{USA}
%   }
% \email{risto@cs.utexas.edu}

% \author{Peter Stone}
% \affiliation{%
%   \institution{The University of Texas at Austin}
%   \institution{and Sony AI}
%   \streetaddress{8600 Datapoint Drive}
%   \city{Austin} \state{Texas} \country{USA}
% %   \postcode{78229}
%   }
% \email{pstone@cs.utexas.edu}

%%
%% By default, the full list of authors will be used in the page
%% headers. Often, this list is too long, and will overlap
%% other information printed in the page headers. This command allows
%% the author to define a more concise list
%% of authors' names for this purpose.
\renewcommand{\shortauthors}{Kumar, et al.}

\maketitle

\appendix

\input{gecco/content/appendix}

%%
%% The next two lines define the bibliography style to be used, and
%% the bibliography file.
% \bibliography{reference.bib}
\bibliographystyle{ACM-Reference-Format}
\bibliography{sample-base}

\end{document}
